# Supplementary material for: RLSbench: Domain Adaptation Under Relaxed Label Shift
Source: arXiv:2302.03020 source file (2023-06-05)
Supplement: Supplementary file 1 [file other_results.tex]

\begin{table}[h!]
    \centering
    \footnotesize
     \setlength{\tabcolsep}{4pt}

        \begin{tabular}{llcccclcccclcccc}
            \toprule
                \multirow{3}{*}{Dataset} & {} &  \multicolumn{4}{c}{\textbf{TENT}} & {} &  \multicolumn{4}{c}{\textbf{DANN}} & {} & \multicolumn{4}{c}{\textbf{NoisyStudent}} \\
                 {} & {}  & \multirow{2}{*}{\parbox{0.5cm}{\centering None}} & {} \multirow{2}{*}{\parbox{0.5cm}{\centering RW}} {} & {} \multirow{2}{*}{\parbox{0.5cm}{\centering RS}} & \multirow{2}{*}{\parbox{0.6cm}{\centering RS+ RW}} & {} & \multirow{2}{*}{\parbox{0.5cm}{\centering None}} & {} \multirow{2}{*}{\parbox{0.5cm}{\centering RW}} {} & {} \multirow{2}{*}{\parbox{0.5cm}{\centering RS}} & \multirow{2}{*}{\parbox{0.6cm}{\centering RS+ RW}} & {} & \multirow{2}{*}{\parbox{0.5cm}{\centering None}} & {} \multirow{2}{*}{\parbox{0.5cm}{\centering RW}} {} & {} \multirow{2}{*}{\parbox{0.5cm}{\centering RS}} & \multirow{2}{*}{\parbox{0.6cm}{\centering RS+ RW}}  \\
                 & & & &&& & & & \\
        \midrule
            cifar10 & {} &  86.8 &       89.9 &     90.7 &          91.8 & {} &  87.0 &       88.2 &     85.6 &          85.5 & {} &          92.2 &               92.3 &             92.2 &                  92.3 \\
           cifar100 & {} &  71.5 &       71.6 &     71.9 &          71.6 & {} &  77.9 &       79.4 &     76.6 &          77.5 & {} &          71.9 &               71.0 &             71.9 &                  71.0 \\
               fmow & {} &  58.0 &       58.2 &     57.8 &          57.8 & {} &  57.8 &       57.9 &     56.8 &          56.6 & {} &          60.6 &               61.1 &             61.0 &                  60.6 \\
           camelyon & {} &  87.3 &       88.5 &     89.4 &          90.4 & {} &  81.2 &       80.9 &     80.4 &          79.8 & {} &          86.0 &               86.0 &             86.4 &                  86.4 \\
          domainnet & {} &  54.1 &       54.2 &     54.4 &          54.2 & {} &  51.8 &       51.8 &     53.5 &          53.2 & {} &          54.4 &               52.4 &             54.3 &                  51.9 \\
           entity13 & {} &  79.6 &       80.8 &     81.0 &          81.9 & {} &  78.4 &       79.5 &     78.6 &          79.8 & {} &          81.2 &               82.1 &             81.6 &                  82.8 \\
           entity30 & {} &  68.5 &       70.1 &     69.3 &          70.9 & {} &  65.8 &       66.9 &     65.4 &          66.9 & {} &          69.7 &               70.0 &             69.4 &                  70.7 \\
           living17 & {} &  71.2 &       71.9 &     71.1 &          72.9 & {} &  68.5 &       71.3 &     70.5 &          71.5 & {} &          74.6 &               74.3 &             71.0 &                  75.9 \\
        nonliving26 & {} &  60.3 &       62.1 &     61.9 &          62.4 & {} &  59.3 &       60.7 &     56.7 &          56.5 & {} &          61.9 &               62.3 &             62.7 &                  63.3 \\
         officehome & {} &  65.6 &       65.8 &     65.8 &          64.9 & {} &  66.5 &       66.6 &     67.7 &          66.7 & {} &          66.7 &               64.7 &             66.8 &                  64.6 \\
              visda & {} &  68.4 &       69.9 &     68.7 &          68.8 & {} &  68.2 &       68.3 &     71.9 &          72.1 & {} &          61.1 &               59.7 &             61.2 &                  59.5 \\
             \midrule
            \textbf{Avg}    & {} &  70.1 &       71.2 &     71.1 &          \textbf{71.6} & {} &  69.3 &       \textbf{70.2} &     69.4 &          69.7 & {} &          \textbf{70.9} &               70.5 &             \textbf{70.8} &                  \textbf{70.8} \\
        \bottomrule
        \end{tabular}

    \caption{\emph{Results with TENT, DANN, and NoisyStudent with re-sampling and re-weighting correction with source validation performance as early stopping criterion aggregated across target label marginal shifts}. 
    Re-sampling and Re-weighting seem to help for all datasets and they both together improve aggregate performance over no correction for all DA methods.}
\end{table}

\begin{table}[h!]
    \centering
    \footnotesize
     \setlength{\tabcolsep}{4pt}

        \begin{tabular}{llcccclcccclcccc}
            \toprule
                \multirow{3}{*}{Dataset} & {} &  \multicolumn{4}{c}{\textbf{TENT}} & {} &  \multicolumn{4}{c}{\textbf{DANN}} & {} & \multicolumn{4}{c}{\textbf{NoisyStudent}} \\
                 {} & {}  & \multirow{2}{*}{\parbox{0.5cm}{\centering None}} & {} \multirow{2}{*}{\parbox{0.5cm}{\centering RW}} {} & {} \multirow{2}{*}{\parbox{0.5cm}{\centering RS}} & \multirow{2}{*}{\parbox{0.6cm}{\centering RS+ RW}} & {} & \multirow{2}{*}{\parbox{0.5cm}{\centering None}} & {} \multirow{2}{*}{\parbox{0.5cm}{\centering RW}} {} & {} \multirow{2}{*}{\parbox{0.5cm}{\centering RS}} & \multirow{2}{*}{\parbox{0.6cm}{\centering RS+ RW}} & {} & \multirow{2}{*}{\parbox{0.5cm}{\centering None}} & {} \multirow{2}{*}{\parbox{0.5cm}{\centering RW}} {} & {} \multirow{2}{*}{\parbox{0.5cm}{\centering RS}} & \multirow{2}{*}{\parbox{0.6cm}{\centering RS+ RW}}  \\
                 & & & &&& & & & \\
                \midrule
                $\infty (\textsc{None})$ & {} &  71.5 &       70.3 &     71.4 &          69.9 & {} &  70.3 &       69.6 &     70.2 &          69.4 & {} &          70.8 &               69.4 &             70.7 &                  69.0 \\
                 10.0 & {} &  71.8 &       70.7 &     72.1 &          70.8 & {} &  70.8 &       70.2 &     70.3 &          69.6 & {} &          70.7 &               69.4 &             71.1 &                  69.6 \\
                  3.0 & {} &  71.3 &       70.6 &     71.5 &          70.4 & {} &  70.3 &       70.4 &     71.0 &          70.3 & {} &          70.8 &               69.6 &             70.7 &                  69.7 \\
                  1.0 & {} &  70.0 &       72.0 &     71.3 &          72.5 & {} &  69.5 &       71.1 &     69.8 &          70.8 & {} &          72.1 &               72.2 &             71.6 &                  72.4 \\
                  0.5 & {} &  66.0 &       70.6 &     69.2 &          72.8 & {} &  65.6 &       69.5 &     65.7 &          68.2 & {} &          70.3 &               72.1 &             69.8 &                  73.4 \\
                 \midrule
                     \textbf{Avg} & {} &  70.1 &       70.8 &     71.1 &          \textbf{71.3} & {} &  69.3 &       \textbf{70.2} &     69.4 &          69.7 & {} &          \textbf{70.9} &               70.5 &             \textbf{70.8} &                  \textbf{70.8} \\
                \bottomrule
                \end{tabular}

    \caption{\emph{Results with TENT, DANN, NoisyStudent with re-sampling and re-weighting correction with source validation performance as early stopping criterion grouped by shift severity}. 
    Re-sampling performs similar or helps across different shifts whereas re-weighting hurts slightly when shift severity is small. However, for severe shifts in target label marginal ($\alpha \in \{1.0, 0.5\}$) re-weighting significantly improves performance.}
\end{table}
