# Supplementary material for: RLSbench: Domain Adaptation Under Relaxed Label Shift
Source: arXiv:2302.03020 source file (2023-06-05)
Supplement: Supplementary file 2 [file all_results.tex]

In this section, we present results across all datasets. 
Different rows show different algorithms and $\{\text{None}, \text{RLLS}, \text{True}\}$ denote the re-weighting estimate used. `None' implies no re-weighting of the classifier. Since IW-CDAN and IW-DAN already incorporate an estimate of target label marginal in their training procedure, we do not adjust the obtained classifier further with our re-weighting correction. 

\begin{table}[h!]
    \centering
    \footnotesize
     \setlength{\tabcolsep}{2.2pt}
     
    % [inline block 0: 11 envs, 53067 chars -> data_tex | \begin{tabular}{llccccccccccccccccccc}     \toprule...]

 
    \caption{Visda results aggregated across different distribution shift pairs}
\end{table}
