# Supplementary material for: RLSbench: Domain Adaptation Under Relaxed Label Shift
Source: arXiv:2302.03020 source file (2023-06-05)
Supplement: Supplementary file 3 [file related.tex]

Tables and figures in the appendix
\begin{itemize}
    \item Dataset tables explaining stats and properties
    \item Tables with all the numbers in appendix
    \item Figures with ranking on individual datasets
    \item Figures with ranking on different alphas aggregated across datasets
    \item Comment on performance with true label shift correction, always improves
    \item Plot showing how label shift simulation increases some divergence!
    \item Add time required to run each methods maybe simply in 1x, 2x and 3x. 
\end{itemize}

\textbf{Other extensions of the label shift setting {} {}}
Several works have tried to relax and extend the label 
shift setting. One line of work extends label shift problem to 
a setting where along with changing prevalance of previously 
unseen classes, novel classes can appear in target~\citep{garg2021PUlearning, garg2022OSLS}. 
On the other hand, label shift setting can also be extended to 
a setting to allow shifts in $p(x|y)$ from source to target. 
This setting has been previously explored as generalized label shift setting 
in 
Kun Zahng's papers on conditional shift. 

Crucially, we are in a different setting.
